# Supplementary material for: A Blind Search for Bursts of Very High Enery Gamma Rays with Milagro
Source: arXiv:0811.1510 source file (2008-11-10)
Supplement: Supplementary file 1 [file AppendixA.tex]

%Appendix
\appendix

\chapter{Overview}
apdxa
